# Supplementary material for: The Standard Model
Source: arXiv:1304.4705 source file (2017-08-25)
Supplement: Supplementary file 1 [file SM._pdf.pdf]

# An Extended Standard Model

W-Y. Pauchy Hwang<sup>1</sup>

*Asia Pacific Organization/Center for Cosmology and Particle Astrophysics,  
Institute of Astrophysics, Center for Theoretical Sciences,  
and Department of Physics, National Taiwan University, Taipei 106, Taiwan*

(April 17, 2013)

## Abstract

Following the thinking underlying the minimal Standard Model, we propose an extended Standard Model, based on the gauge group  $SU_c(3) \times SU_L(2) \times U(1) \times SU_f(3)$ . The extension, which is rather unique, derives from the family concept that there are three generations of quarks and of leptons. It yields neutrino oscillations in a natural manner. It also predicts a variety of lepton-flavor-violating rare decays.

PACS Indices: 12.60.-i (Models beyond the standard model); 98.80.Bp (Origin and formation of the Universe); 12.10.-g (Unified field theories and models).

Nowadays it is firmly established that there are three generations of quarks and of leptons, at the level of the so-called "point-like Dirac particles". According to another newly established belief in Cosmology, the content of the current Universe would be 25 % in the dark matter while only 5% in the ordinary matter, the latter described by the "minimal Standard Model" (mSM). The dark-matter particles are supposed to be described by an extended Standard Model. Thus, there is certain urgent need for an extended Standard Model, which accommodates those phenomena which are "beyond the Standard Model".

In the attempt to write down another extended Standard Model, we would try to write it as a whole - strong interactions, electroweak interactions, and others as a whole, and not separately. In that way, the "basic units", which are based on the right-handed Dirac components or left-handed Dirac components, would be more appropriate than just "the building blocks of matter". Each basic unit derives from one kinetic-energy term,  $-\bar{\Psi}_R \gamma_\mu \partial_\mu \Psi_R$  or  $-\bar{\Psi}_L \gamma_\mu \partial_\mu \Psi_L$ , and from only one such term. The gauge principle tells us that  $\partial_\mu$  is to be replaced by some "gauge-invariant" derivative  $D_\mu$ . This would be a way to write down a theory in the globally consistent manner.

We may split the ordinary-matter world into the "quark" world and the "lepton" world. As we know so far, the dark-matter world does not involve *directly* strong and electromagnetic interactions. We could decide which multiplet of the dark-matter group  $SU_f(3)$  each basic unit should belong - for instance, we may rule out the direct coupling between the quark world and the dark-matter world, altogether.

How about the couplings between the family group  $SU_f(3)$  and the lepton world? We know that the right-handed neutrinos do not appear in the minimal Standard Model - so,  $(\nu_{\tau R}, \nu_{\mu R}, \nu_{e R})$  would make a perfect triplet under  $SU_f(3)$ . In a recent note [1], we proposed to put  $((\nu_\tau, \tau)_L, (\nu_\mu, \mu)_L, (\nu_e, e)_L)$  (*columns*) ( $\equiv \Psi_L(3, 2)$ ) as the  $SU_f(3)$  triplet and  $SU_L(2)$  doublet. The next question is how to assign  $\tau_R, \mu_R$ , and  $e_R$  under  $SU_f(3)$ . We

---

<sup>1</sup>Correspondence Author; Email: wyhwang@phys.ntu.edu.tw; arXiv:1304.xxxx [hep-ph] 17 April 2013.

could write down the mass term for the charged leptons - if they are singlets or  $(\tau_R, \mu_R, e_R)$  is an  $SU_f(3)$  triplet? The singlet assignment can be ruled out since there are undesirable crossed terms in, e.g.,  $\Psi_L(\bar{3}, 2)e_R\Phi(3, 2)$ . So, three of them would form a triplet -  $\Psi_R^C(3, 1)$ . In fact, this would imply that three charged leptons would have equal masses, to the zeroth order. Or, we go back to the ground-zero: the  $SU_f(3)$  is completely decoupled. Nevertheless, it might not be so bad to have the beginning point that we have to look for why the three charged leptons have different masses. This would complete the list of "the basic units".

So, there are only three members in the lepton world - two right-handed triplets and one "composite" left-handed triplet under  $SU_f(3)$ . It is rather simple if we wish to play with  $SU_f(3)$ .

Since we wish to propose the  $SU_f(3)$  family gauge theory as a way to understand why there are three generations, it requires all additional particles, i.e., (eight) gauge bosons and (four) residual family Higgs, very massive. In the proposal of Hwang and Yan [1], we would have one Standard-Model Higgs field  $\Phi(1, 2)$ , one complex family Higgs triplet  $\Phi(3, 1)$ , and another family triplet-doublet complex scalar fields  $\Phi(3, 2)$ . Amazingly enough [2], two neutral complex triplets,  $\Phi(3, 1)$  and  $\Phi^0(3, 2)$  would indeed undergo the desired Higgs mechanism and the three charged scalar fields would remain massive, i.e. there is no spontaneous symmetry breaking (SSB) in the charged Higgs sector.

So far, we have decided on the basic units - those left-handed and right-handed quarks and leptons; the gauge group is chosen to be  $SU_c(3) \times SU_L(2) \times U(1) \times SU_f(3)$ . For notations, we use Wu and Hwang [3].

In the quark world, we have, for the up-type right-handed quarks  $u_R, c_R$ , and  $t_R$ ,

$$D_\mu = \partial_\mu - ig_c \frac{\lambda^a}{2} G_\mu^a - i \frac{2}{3} g' B_\mu, \quad (1)$$

and, for the rotated down-type right-handed quarks  $d'_R, s'_R$ , and  $b'_R$ ,

$$D_\mu = \partial_\mu - ig_c \frac{\lambda^a}{2} G_\mu^a - i \left(-\frac{1}{3}\right) g' B_\mu. \quad (2)$$

On the other hand, we have, for the  $SU_L(2)$  quark doublets,

$$D_\mu = \partial_\mu - ig_c \frac{\lambda^a}{2} G_\mu^a - ig \frac{\vec{\tau}}{2} \cdot \vec{A}_\mu - i \frac{1}{6} g' B_\mu. \quad (3)$$

In the lepton world, we introduce the family triplet,  $(\nu_\tau^R, \nu_\mu^R, \nu_e^R)$  (column)  $(\equiv \Psi_R(3, 1))$ , under  $SU_f(3)$ . Since the minimal Standard Model does not see the right-handed neutrinos, it would be a natural way to make an extension of the minimal Standard Model. Or, we have, for the triplet  $(\nu_\tau^R, \nu_\mu^R, \nu_e^R)$ ,

$$D_\mu = \partial_\mu - i\kappa \frac{\bar{\lambda}^a}{2} F_\mu^a. \quad (4)$$

and, for the left-handed  $SU_f(3)$ -triplet and  $SU_L(2)$ -doublet  $((\nu_\tau^L, \tau^L), (\nu_\mu^L, \mu^L), (\nu_e^L, e^L))$  (all columns)  $(\equiv \Psi_L(3, 2))$ ,

$$D_\mu = \partial_\mu - i\kappa \frac{\bar{\lambda}^a}{2} F_\mu^a - ig \frac{\vec{\tau}}{2} \cdot \vec{A}_\mu + i \frac{1}{2} g' B_\mu. \quad (5)$$

As discussed earlier, it follows as the only option that three of the right-handed charged leptons have to form an  $SU_f(3)$  triplet  $\Psi_R^C(3, 1)$ .

The generation of the various quark masses is through the Standard-Model way. For the charged leptons, we have to choose  $\bar{\Psi}_L(\bar{3}, 2)\Psi_R^C(3, 1)\Phi(1, 2)$ . Note that, in the U-gauge, the SM Higgs looks like  $(0, \frac{1}{\sqrt{2}}(v + \eta(x)))$ , only one degree of freedom [3]. Thus, the neutral neutrino triplet  $\Psi_R(3, 1)$  cannot be used in the above coupling, because of the charge conservation.

For neutrinos in the lepton world, the neutrino mass term becomes [1, 2]

$$i\frac{\eta}{2}\bar{\Psi}_L(3, 2) \times \Psi_R(3, 1) \cdot \Phi(3, 2) + h.c.. \quad (6)$$

The cross (curl) product is somewhat new [4], referring to the singlet combination of three triplets in  $SU(3)$  - suitable for  $SU(3)$ ; *not* an ordinary matrix operation. In this note, we are careful enough to distinguish the anti-triplet from the triplet and to realize that there are a lot of "conjugates", such as "complex conjugate", "Dirac adjoint", and "anti-triplet" (though sometime the same).

The last expression serves as the operator describing neutrino oscillations in general. For point-like Dirac particles, this way of describing oscillations is rather natural and unique.

To summarize on the origin of masses, the quark masses are determined by the vacuum expectation values (VEV's) of the SSB of the Standard-Model Higgs  $\Phi(1, 2)$  and of the adjoint, the charged lepton mass is determined *cooperatively* by  $\Phi(1, 2)$ , while the neutrino masses are determined by the purely and mixed family Higgs  $\Phi(3, 1)$  and  $\Phi^0(3, 2)$  (neutral). In the leading order, the equality of the three charged leptons remains to be explained - presumably by higher-order loop diagrams.

To be more precise, our gauge group is  $(SU_c(3) \times SU_L(2) \times U(1)) \times SU_f(3)$ , rather than  $SU_c(3) \times SU_L(2) \times U(1) \times SU_f(3)$ . That is why it is so difficult to find.

As pointed out in an early paper [2], we may imagine that, in the U-gauge, the standard-model Higgs  $\Phi(1, 2)$  looks like  $(0, (v + \eta(x))/\sqrt{2})$  (*column*) and  $\Phi^\dagger(\bar{3}, 2)\Phi(1, 2)$  would pick out the neutral sector naturally. In fact, the term  $(\Phi^\dagger(\bar{3}, 2)\Phi(1, 2))(\Phi^\dagger(1, 2)\Phi(3, 2))$  with a suitable sign, would modify a massive  $\Phi(3, 2)$  field such that the neutral sector has SSB while the charged sector remains massive. This "project-out" Higgs mechanism is what we need.

We may [2] write down the terms for potentials among the three Higgs fields, subject to (1) that they are renormalizable, and (2) that symmetries are only broken spontaneously (via the Higgs or induced Higgs mechanism). We write [2]

$$V = V_{SM} + V_1 + V_2 + V_3, \quad (7)$$

$$\begin{aligned} V_1 = & \frac{M^2}{2}\Phi^\dagger(\bar{3}, 2)\Phi(3, 2) + \frac{\lambda_1}{4}(\Phi^\dagger(\bar{3}, 2)\Phi(3, 2))^2 \\ & + \epsilon_1(\Phi^\dagger(\bar{3}, 2)\Phi(3, 2))(\Phi^\dagger(1, 2)\Phi(1, 2)) + \eta_1(\Phi^\dagger(\bar{3}, 2)\Phi(1, 2))(\Phi^\dagger(1, 2)\Phi(3, 2)) \\ & + \epsilon_2(\Phi^\dagger(\bar{3}, 2)\Phi(3, 2))(\Phi^\dagger(\bar{3}, 1)\Phi(3, 1)) + \eta_2(\Phi^\dagger(\bar{3}, 2)\Phi(3, 1))(\Phi^\dagger(\bar{3}, 1)\Phi(3, 2)) \\ & + (\delta_1 i \Phi^\dagger(3, 2) \times \Phi(3, 2) \cdot \Phi^\dagger(3, 1) + h.c.), \end{aligned} \quad (8)$$

$$V_2 = \frac{\mu_2^2}{2}\Phi^\dagger(\bar{3}, 1)\Phi(3, 1) + \frac{\lambda_2}{4}(\Phi^\dagger(\bar{3}, 1)\Phi(3, 1))^2 + (\delta_2 i \Phi^\dagger(3, 1) \cdot \Phi(3, 1) \times \Phi(3, 1) + h.c.)$$

$$V_3 = +\lambda'_2 \Phi^\dagger(\bar{3}, 1) \Phi(3, 1) \Phi^\dagger(1, 2) \Phi(1, 2), \quad (9)$$

$$+ (\delta_3 i \Phi^\dagger(3, 2) \cdot \Phi(3, 2) \times (\Phi^\dagger(1, 2) \Phi(3, 2)) + h.c.) \\ + (\delta_4 i (\Phi^\dagger(3, 2) \Phi(1, 2)) \cdot \Phi^\dagger(3, 1) \times \Phi(3, 1) + h.c.) \\ + \eta_3 (\Phi^\dagger(\bar{3}, 2) \Phi(1, 2) \Phi(3, 1) + c.c.). \quad (10)$$

We maintain that every terms are naively renormalizable since they are of power four or less. Note that the terms in  $\delta_i i$  involve the so-called " $SU(3)$  operations", as before.

In the simplest case, we could assume

$$M^2 > 0, \quad \lambda_1 > 0, \quad \eta_1 \neq 0, \quad \eta_2 \neq 0, \\ \mu_2^2 < 0, \quad \lambda_2 > 0, \\ \text{all other couplings vanish.} \quad (11)$$

In the present case, we require  $M^2 + \eta_1 v^2/2 < 0$  to ensure that SSB takes place in the neutral sector of  $\Phi(3, 2)$ . The cross term in  $\eta_2$  might be optional (i.e. with other options) since we follow the early paper [5] on the colored Higgs mechanism to absorb the four DOF's from one complex triplet.

So, we see that, at the Lagrangian level, the  $SU_c(3) \times SU_L(2) \times U(1) \times SU_f(3)$  gauge symmetry is protected but such symmetry is violated via spontaneous symmetry breaking (via the SM Higgs mechanism and the project-out Higgs mechanism).

The scenario for the masses of the family particles might be as follows: For those eight familons (or family gauge bosons), we could assume a few  $TeV$  or slightly more. For those four family Higgs (those participating Higgs mechanisms), maybe even slightly more heavier. We don't have definitive expectations for the charged scalar particles, except that they could be much heavier.

We note that the terms allowed by the renormalizability, in  $V_1$ ,  $V_2$ , and  $V_3$  given above, are rather rich. This is the nature of the scalar fields and their vacuum expectation values.

As shown earlier [4, 5], two triplets of complex scalar fields would make the eight family gauge bosons and four residual family Higgs particles all massive, presumably heavier than a few  $TeV$ . In the  $SU_f(3)$  family gauge theory treated alone, there are many ways of accomplishing such goal. In the present complicated case, the equivalence between two triplets is lost, but presumably in a minor way.

Neutrinos have tiny masses far smaller than the masses of the quarks or of charged leptons. Neutrinos oscillate among themselves, giving rise to the lepton-flavor violation (LFV). There are other oscillation stories, such as the oscillation in the  $K^0 - \bar{K}^0$  system, but there is a fundamental "intrinsic" difference here - the  $K^0 - \bar{K}^0$  system is composite while neutrinos are regarded as "point-like" Dirac particles. We could draw Feymann diagrams for the oscillating  $K^0 - \bar{K}^0$  system; but none so far on neutrino oscillations. It is fair to say that neutrino masses and neutrino oscillations may be regarded as one of the most important experimental facts over the last thirty years [6].

In fact, certain LFV processes such as  $\mu \rightarrow e + \gamma$  [6] and  $\mu + A \rightarrow A^* + e$  are closely related to the most cited picture of neutrino oscillations so far [6]. In recent publications [7], it was pointed out that the cross-generation or off-diagonal neutrino-Higgs interaction may serve as the detailed mechanism of neutrino oscillations, with some vacuum expectation value(s)

of the new Higgs fields,  $\Phi(3,1)$  and  $\Phi^0(3,2)$ . *So, even though we haven't seen, directly, the family gauge bosons and family Higgs particles, we already see the manifestations of their vacuum expectation values.*

In the other words, Eq. (6), the  $SU(3)$ -generalized curl product, can be used as the basis to analyze the various lepton-flavor-violating decays and reactions, in addition to its implications on the tiny neutrino masses and on neutrino oscillations.

To close this note, We would like to speculate what the dark-matter world look like, if the extended Standard Model discussed is true.

In a slightly different context [8], it was proposed that we could work with two working rules: "Dirac similarity principle", based on eighty years of experience, and "minimum Higgs hypothesis", from the last forty years of experience. Using these two working rules, the extended model mentioned above becomes rather unique - so, it is so much easier to check it against the experiments. These two working rules merely assert that our world is rather simple.

We would be curious about how the dark-matter world looks like, though it is difficult to verify experimentally. The first question would be: The dark-matter world, 25 % of the current Universe (in comparison, only 5 % in the ordinary matter), would clusterize to form the dark-matter galaxies, maybe even before the ordinary-matter galaxies. The dark-matter galaxies would then play the hosts of (visible) ordinary-matter galaxies, like our own galaxy, the Milky Way. Note that a dark-matter galaxy is by our definition a galaxy that does not possess any ordinary strong and electromagnetic interactions (with our visible ordinary-matter world). This fundamental question deserves some thoughts, for the structural formation of our Universe.

Of course, we should remind ourselves that, in our ordinary-matter world, those quarks can aggregate in no time, to hadrons, including nuclei, and the electrons serve to neutralize the charges also in no time. Then atoms, molecules, complex molecules, and so on. These serve as the seeds for the clusters, and then stars, and then galaxies, maybe in a time span of  $1\text{ Gyr}$  (i.e., the age of our young Universe). The aggregation caused by strong and electromagnetic forces is fast enough to help giving rise to galaxies in a time span of  $1\text{ Gyr}$ . On the other hand, the seeded clusterings might proceed with abundance of extra-heavy dark-matter particles such as familons and family Higgs, all greater than a few  $\text{TeV}$  and with relatively long lifetimes (owing to very limited decay channels). So, further simulations on galactic formation and evolution may yield clues on our problem.

This work is supported in part by the National Science Council (NSC99-2112-M-002-009-MY3).

## References

- [1] W-Y. Pauchy Hwang and Tung-Mow Yan, arXiv:1212.4944 [hep-ph] 20 Dec 2012.
- [2] W-Y. Pauchy Hwang, arXiv:1301.6464v3 [hep-ph] 10 April 2013.
- [3] Ta-You Wu and W-Y. Pauchy Hwang, "Relativistic Quantum Mechanics and Quantum Fields" (World Scientific 1991).

- [4] W-Y. Pauchy Hwang, Nucl. Phys. **A844**, 40c (2010); *ibid.*, International J. Mod. Phys. **A24**, 3366 (2009); *ibid.*, Intern. J. Mod. Phys. Conf. Series **1**, 5 (2011); *ibid.*, American Institute of Physics 978-0-7354-0687-2/09, pp. 25-30 (2009).
- [5] W-Y. P. Hwang, Phys. Rev. **D32**, 824 (1985).
- [6] Particle Data Group, "Review of Particle Physics", J. Phys. G: Nucl. Part. Phys. **37**, 1 (2010); and its biennial publications.
- [7] W-Y. Pauchy Hwang, arXiv:1207.6443v1 [hep-ph] 27 Jul 2012; *ibid.*, Hypefine Interactions **215**, 105 (2013); *ibid.*, arXiv:1209.5488v1 [hep-ph] 25 Sep 2012.
- [8] W-Y. P. Hwang, arXiv:11070156v1 (hep-ph, 1 Jul 2011), Plenary talk given at the 10th International Conference on Low Energy Antiproton Physics (Vancouver, Canada, April 27 - May 1, 2011).
